# Supplementary material for: Large Deviation Theory for Parameter Estimation in Simple Neuron Models
Source: arXiv:1707.04648 source file (2017-07-14)
Supplement: Supplementary file 1 [file AppendixA.tex]

% Appendix A
\newgeometry{textwidth=17cm}%,textheight=10cm}
\chapter{\texttt{R} source code} % Main appendix title
\label{AppendixA} % For referencing this appendix elsewhere, use \ref{AppendixA}
\begin{multicols}{2}
\begin{minted}[fontsize=\scriptsize,breaklines]{R}
library(Sim.DiffProc)
library(tictoc)
library(FNN)

# Parameters according to Lansky, Sanda and He (2006)
# m should be bigger than 500
m <- 5000; n <- 5000;
theta <- 25.8042;
mu <- 0.341/theta;
epsilon <- 0.0114;
x0 <- mu; T <- 5;

# Prepare expressions for SDE
f <- expression( -theta*(x-mu) )
g <- expression( epsilon )

# Interesting values for the constant boundary
L2 <- seq(0.013,0.017,0.0005);

# Prepare lists
means <- c()
means_alt <- c()
store_boundaries <- c()
store_boundaries_alt <- c()

##
# For all values of the boundary simulate SDE with Runge-Kutta scheme
# Not efficient but safe
for(l in L2){
  print(l)
  St <- as.expression(l) 
  # Takes time
  tic()
  res1 <- fptsde1d(N=n, M=m, drift=f, diffusion=g, boundary=St,  x0=0, T=T, method = "rk3")
  toc()
  tic()
  res2 <- fptsde1d(N=n, M=m, drift=f, diffusion=g, boundary=St,  x0=x0, T=T, method = "rk3")
  toc()
  # Store and summarize
  store_boundaries <- cbind(store_boundaries , res1)
  store_boundaries_alt <- cbind(store_boundaries_alt , res2)
  means <- cbind(means,mean(res1))
  means_alt <- cbind(means_alt , mean(res2))
  summary(res1)
}
## Display them all
redts <- ts(res1$SDE$X[,1:200] , start=res1$SDE$t0, end=res1$SDE$T, deltat=res1$SDE$Dt)
plot(redts, plot.type="single", col=c("red","blue","orange"), type="l",ylab="Voltage", ,cex.axis=1.5,cex.lab=2, cex.main=2)

##
# Transition Histograms
my_mat <- matrix(res1$SDE$X , ncol = m)
# Plot histograms and predicted densities
# Select interesting points in time
Ts <- c(0.005,0.01,0.05,3)
par(mfrow=c(1,4),mar = c(5,5,4,2)+0.1)
for(T1 in Ts){
  # Round the selected timepoint so that it corresponds to a simulated one
  idx <- floor((T1 * nrow(my_mat))/T)
  T2 <- idx*(T/n)
  print(idx)
  # Calculate theoretical parameters and distribution
  mean <- mu - mu*exp(-theta*T2)
  sd <- sqrt((epsilon^2/(2*theta))* (1-exp(-2*theta*T2)))
  dx <- seq(from=mean - 5*sd,to=mean + 5*sd,length.out=1000)
  px <- dnorm(seq(from=mean - 5*sd,to=mean + 5*sd,length.out=1000), mean = mean, sd = sd)
  # Plot simulated histogram
  hist(my_mat[idx,],freq=FALSE,
       xlab="Voltage",breaks=15,
       main=paste("T = ",T1),
       ylim=c(0,max(px)+20), cex.axis=1.5, cex.lab=2, cex.main=2)
  # Overlay theoretical distribution 
  lines(dx,
        px, lwd=5,
        col="red")
}
## Calculate KL divergence assuming that simulated data comes from a
## gaussian normal distribution with the estimated parameters
T2s = seq(0.005,0.2,0.007)
KLs <- c()
for(T1 in T2s){
  # Round as above
  idx <- floor((T1 * nrow(my_mat))/T)
  T2 <- idx*(T/n)
  print(idx)
  # Predicted and estimated
  mean <- mu - mu*exp(-theta*T2)
  sd <- sqrt((epsilon^2/(2*theta))* (1-exp(-2*theta*T2)))
  # KL divergence for two Gaussians
  KLs <- cbind(KLs, log(sd(my_mat[idx,])/sd) + 
                 (sd^2 + (mean - mean(my_mat[idx,]))^2) /(2*sd(my_mat[idx,])^2) -0.5
  )
}
# Plot in single figure
par(mfrow=c(1,1))
plot(T2s,KLs[1,],ylab="KL divergence", xlab="Time", cex.axis=1.5, cex.lab=2, cex.main=2)

## 
# FPT historgrams

#Plotting setup (Big plot - zoom into figure!)
laymat <- matrix(c(1,2,3,4,5,6,7,8,9,10,10,10),nrow = 4,ncol = 3,byrow = TRUE)
layout(mat = laymat)
#Kullback Leibler Divergences
KLs <- c()
##
# For all boundary values estimate KL divergence between the two initial conditions
for(i in seq(1,length(L2))){
  # KL estimation with k nearest neighbors density estimation
  set1 <- store_boundaries[,i]$fpt
  set2 <- store_boundaries_alt[,i]$fpt
  KLval <- KLx.divergence(set2[!is.na(set2)], set1[!is.na(set1)],k=50)
  KLs <- cbind(KLs,KLval[1])
  # Plot 2 Histograms in one subplot
  h1 <- hist(set1,breaks=50,plot=FALSE)
  h2 <- hist(set2,breaks=50,plot=FALSE)
  plot( h2,xlab = "Time", col="gray", cex.axis=1.5, cex.lab=2, cex.main=2,
        main=paste("Boundary ",L2[i]))#, xlim=c(0,10))  # first histogram
  par(new=TRUE)
  plot( h1, col=rgb(1,0,0,1/4), add=T)
}
# Add legend underneath
plot(1, type = "n", axes=FALSE, xlab="", ylab="")
plot_colors <- c("red","grey")
legend(x = "top", pt.cex=c(5,5), cex=2.5, pch=c(15,15), 
       legend = c("Start at reset value", "Start in equilibrium"), 
       col=plot_colors, horiz = TRUE,bty='n')
# Display KL divergences
print(KLs)
par(mfrow=c(1,1),mar = c(5,5,4,2)+0.1)
plot(L2 , KLs , ylab="KL divergence",cex.axis=1.5,cex.lab=2, cex.main=2)

##
# Plot theoretical Eyring-Kramer estimate and Kramer Estimate
dx <- seq(0.013,0.045,0.001)
par(mar = c(5,5,4,2)+0.1)
plot(dx , exp((theta/epsilon)* (dx-mu)^2), type="l", col="orange",  lwd=5, ylab="EFPT", xlab="Offset", ylim=c(0,3), cex.axis=1.5, cex.lab=2, 
     cex.main=2)
# Eyring-Kramer law
lines(dx , (2*pi/theta)* exp((theta/epsilon)*(dx-mu)^2), type="l",
      lwd=5, col="red")


## Compare with simulated means
means <- c()
means_alt <- c()
for (i in seq(length(L2))) {
  temp <- store_boundaries[,i]$fpt
  temp2 <- store_boundaries_alt[,i]$fpt
  means <- cbind(means , mean(temp[!is.na(temp)]))
  means_alt <- cbind(means_alt , mean(temp2[!is.na(temp2)]))
}

# Kramer's law
plot(L2 , exp((theta/epsilon)* (L2-mu)^2), type="l", col="orange", lwd=5, ylab="EFPT",xlab="Offset", ylim=c(0,1.5), cex.axis=1.5,cex.lab=2, cex.main=2)
# Eyring-Kramer law
lines(L2 , (2*pi/theta)* exp((theta/epsilon)*(L2-mu)^2), type="l",
      lwd=5 ,col="red")
# Simulated values
lines(L2,means,col="blue",type="o")
lines(L2,means_alt,col="green",type="o")

legend("topleft",c("Simulated from reset","Simulated from equilibrium","Kramer's","Eyring-Kramer"), col=c("blue","green","orange","red"), lty=c(1,1))

# Fit quadratic model to the logarithm of the data
model <- lm(log(c(means)) ~ I(L2^2))#poly(L2,2))
print(confint(model))
predicted.intervals <- predict(model, data.frame(x=L2), interval='confidence', level=0.95)
plot(L2, predicted.intervals[,1], col='blue',lwd=3,type='l', ylab='log(EFPT)' ,cex.axis=1.5, cex.lab=2, cex.main=2)
lines(L2,predicted.intervals[,2],col='black',lwd=1)
lines(L2,predicted.intervals[,3],col='black',lwd=1)
lines(L2,log(means),col='green',lty=2,type='p',lwd =3)

legend("topleft",c("Simulated","LS polynomial curve","Confidence bounds"), col=c("green","blue","black"), lty=c(2,1,1),cex=1.5)

# Fit quadratic model to the logarithm of the data
model <- lm(log(c(means_alt)) ~ I(L2^2))#poly(L2,2))
print(confint(model))
predicted.intervals <- predict(model,data.frame(x=L2), interval='confidence', level=0.95)
plot(L2,predicted.intervals[,1], col='blue', lwd=3, type='l', ylab='log(EFPT)' ,cex.axis=1.5, cex.lab=2, cex.main=2)
lines(L2,predicted.intervals[,2],col='black',lwd=1)
lines(L2,predicted.intervals[,3],col='black',lwd=1)
lines(L2,log(means_alt),col='green',lty=2,type='p',lwd =3)

legend("topleft",c("Simulated","LS polynomial curve","Confidence bounds"), col=c("green","blue","black"), lty=c(2,1,1),cex=1.5)
\end{minted}
\end{multicols}
\restoregeometry
